# Supplementary material for: Argue with Me Tersely: Towards Sentence-Level Counter-Argument Generation
Source: arXiv:2312.13608 source file (2023-12-21)
Supplement: Supplementary file 1 [file temp6.tex]

\section{More Information about the Annotation Process}
\label{annotation process}

The dataset was enhanced through thorough annotation of the CMV dataset. Within CMV, a quoting dynamic exists: user B selects a part of user A's statement (usually a sentence) and responds to it (often multiple sentences). These sentence pairs with quoting relations were defined as "conversations," serving as annotation source data. User A's statement is the original argument, and annotators extract concise expressions (single sentence) from user B's replies as sentence-level counter-argument.

Before presenting conversations and topics to annotators, we preprocessed the source data. User B's replies were segmented into candidate sentences using punctuation marks, and sentences containing hyperlinks, emails, phone numbers, emojis, etc., were removed (which protects the privacy of users). After that, grammar errors (capitalization, spacing) were corrected.

Annotators selected sentences from the candidate set that convincingly refuted the original argument. An option to invalidate conversations was provided, applicable if the original argument was syntactically incomplete, lacked a specific viewpoint, or contained harmful content.

Prior to formal annotation, annotators underwent training which included understanding annotation rules and the system, as well as sensitivity towards invalidating conversations. After training, annotators conducted trial annotations. Consistency between our self-annotations and each annotator's results was assessed, retaining those with good consistency for formal annotation (24 annotators at last). During formal annotation, two annotators cross-evaluated each content piece. If a candidate sentence was unanimously selected or not by both annotators, it became a sentence-level counter-argument. Otherwise, a third annotator arbitrated and determined the final result. About 30\% of the corpus is generated by arbitration. Invalid conversations were promptly removed during the annotation process if an annotator deemed them unfit. The annotation process lasted 42 days.
